# Supplementary material for: CMB Tensor Anisotropies in f(R) Gravity
Source: arXiv:1302.1887 source file (2013-02-07)
Supplement: Supplementary file 1 [file sigma2u.tex]

\documentclass[a4paper,12pt]{article}
\usepackage[utf8x]{inputenc}
\usepackage{amssymb}
\usepackage{amsmath}

%opening
\title{Wave Eq.: From $\sigma$ to $u$}
\author{Hassan Bourhrous}

\begin{document}

%%%%%%%%%%%%%%%%%%%% % Bourhrous % %%%%%%%%%%%%%%%%%%%%%%
\def \vec #1{\textbf{\em  #1}}
\newcommand{\Cl}{C_\ell}
\newcommand{\Pl}{P_\ell}
\newcommand{\cn}{/**citation needed**/}
%\newcommand{\l}{\ell}
%%%%%%%%%%%%%%%% % Leong % %%%%%%%%%%%%%%%%

\newcommand{\p}{\partial}
\newcommand{\D}{\Delta}
\newcommand{\n}{\nabla}
\def\l{\left}
\def\r{\right}
\def\D{\Delta}
\def\dt{\cdot}
\def\w{\wedge}
\def\n{\nabla}
\newcommand{\hs}{\,-\,}
\newcommand \dd[2] {\frac{d {#1}}{d {#2}}}
\newcommand \pp[2] {\frac{\p {#1}}{\p {#2}}}
\newcommand \ppd[2] {\frac{\p^2 {#1}}{\p {#2}^2}}
\newcommand \ddp[2] {\frac{ d^2 {#1}}{d {#2}^2}}
\newcommand \bra[1] {\big< {#1}|}
\newcommand \ket[1] {| {#1} \big>}
\newcommand \ps {\mathcal{I}}
\newcommand{\nab}{\tilde{\nabla}}
\renewcommand{\theequation}{\arabic{equation}}
\def\mat#1  { \begin{matrix}#1\end{matrix} }
\def\pmat#1 { \begin{pmatrix}#1\end{pmatrix} }
\def\cas#1  { \begin{cases}#1\end{cases} }

%%%%%%%%%%%%%%%%% Commands from Ananda et. al %%%%%%%%%%%%
% 

\def \D {\tilde{\nabla}}
\def \ni {\noindent}
\def\3nab{\tilde{\nabla}}
\def\lgl{\langle}
\def\rgl{\rangle}
\def\nn{\nonumber}
\def\c{\mbox{curl}}
\newcommand{\curl}{\,\mbox{curl}\,}
\newcommand{\Drm}{{\mathrm{D}}}

\maketitle

\section{Wave Equation in $f(R)$}

We start from this verified equation for the shear:
\begin{equation}
\ddot \sigma_{ab} - \D^2 \sigma_{ab}  + \frac{5}{3} \, \Theta \, \dot \sigma_{ab} + \l( \frac{1}{2} \rho - \frac{3}{2} p 
\r) \, \sigma_{ab} = \dot \pi_{ab} + \frac{2}{3} \, \Theta \, \pi_{ab} 
\label{gws}
\end{equation}
Expanding into tensor harmonics:
\begin{align}
E_{ab} &= \sum_{k} \l( \frac{k}{a} \r)^2 \l[ E_k Q_{ab}^{(k)} + \bar E_k \bar Q_{ab}^{(k)} \r] \\ 
H_{ab} &= \sum_{k} \l( \frac{k}{a} \r)^2 \l[ H_k Q_{ab}^{(k)} + \bar H_k \bar Q_{ab}^{(k)} \r] \\ 
\sigma_{ab} &= \sum_{k} \frac{k}{a} \l[ \sigma_k Q_{ab}^{(k)} + \bar \sigma_k \bar Q_{ab}^{(k)} \r] \\
\pi_{ab} &= \rho \sum_{k} \l[ \pi_k Q_{ab}^{(k)} + \bar \pi_k \bar Q_{ab}^{(k)} \r]
\end{align}
and using:

\begin{equation}
\pi_{ab} = \frac{\pi_{ab}^m}{f_R} + \pi_{ab}^R, \label{anis_decomp}
\end{equation}
where
\begin{equation}
\pi^{R}_{ab} = \frac{1}{f_R} \left[ f_{2R}\D_{\lgl a}\D_{b\rgl}R+f_{3R}\D_{\lgl a}{R}\D_{b\rgl}{R}-f_{2R} \, \sigma_{ab}\dot{R} \right]
\end{equation}
we get, to first order:
\begin{equation}
\ddot \sigma_k + A \dot \sigma_k + B \sigma_k = \frac{a}{k} \frac{\rho}{f_R} \l[ \dot \pi^\gamma_k - \l( H + 3H\omega +
\frac{f_{2R}}{f_R} \r) \pi^\gamma_k \r] 
\end{equation}
with $$A = 3H + \frac{f_{2R}}{f_R} \dot R$$ and $$B = \frac{k^2}{a^2} + 2 \frac{\ddot a}{a} + \dot R^2 \l( \frac{f_{3R}}{f_R} -\l(
\frac{f_{2R}}{f_R} \r) ^2 \r) + \frac{f_{2R}}{f_R} \ddot R + H \frac{f_{2R}}{f_R} \dot R $$

Neglecting the radiation anisotropic stress and changing to conformal time:

\begin{equation}
\sigma_k '' + \l( a A - \mathcal{H} \r) \sigma_k ' + a^2 B \sigma_k =  0
\label{shear_wave_eq_eta}
\end{equation}

Making the variable change $u_k = a^m \sigma_k$ and choosing $m = \frac{Aa - \mathcal{H}}{2 \mathcal{H}}$, Eq.
(\ref{shear_wave_eq_eta}) becomes:

\begin{equation}
u_k '' + \l[ - \frac{1}{2} m \mathcal{H} \frac{f_{2R}}{f_R} R' - m \frac{a''}{a} + a^2 B \r] u_k = 0
\label{uwave}
\end{equation}

\section{$f(R) = R^n$}

$$R = 6 \frac{a''}{a^3}$$

Introducing the parameter \hspace{0.5cm} $\varepsilon \equiv \frac{2n}{3(1 + \omega)} -1 $ \hspace{0.5cm} such that \hspace{0.5cm} $a(\eta) = \eta^{-\frac{1+\varepsilon}{\varepsilon}}$

m becomes $$m = 1 + \frac{1-n}{1+\varepsilon}$$

Working out the terms of Eq.(\ref{uwave}) in $f(R) = R^n$:

\begin{align}
& \frac{f_{2R}}{f_R} = (n-1) R^{-1}\\
& \frac{f_{3R}}{f_R} = (n-1)(n-2) R^{-2} \\
& \mathcal{H} = - \frac{\varepsilon + 1}{\varepsilon} \eta^{-1} \\
& R = 6 \frac{(\varepsilon+1)(2 \varepsilon + 1)}{\varepsilon^2} \eta^\frac{2}{\varepsilon} \\
& R' = 12 \frac{(\varepsilon+1)(2 \varepsilon + 1)}{\varepsilon^3} \eta^\frac{2-\varepsilon}{\varepsilon} \\
& R'' = 6 \frac{(\varepsilon+1)(2 \varepsilon + 1)(2-\varepsilon)}{\varepsilon^4} \eta^\frac{2-2\varepsilon}{\varepsilon} \\
& a A = \frac{1}{\varepsilon} \l( 2(n-1) -3(\varepsilon+1) \r) \eta^{-1}\\
& a^2 B = k^2 + 2 m \l( \frac{\varepsilon +1}{\varepsilon} \r) \eta^{-2}
\end{align}
I have more details about this on paper if you want to discuss it.

Equation \eqref{uwave} becomes:
\begin{equation}
u_k'' + \l[k^2 + m \l( \frac{\varepsilon + 1}{\varepsilon^2} \r) \l( n-2 \r) \eta^{-2} \r] u_k = 0
\label{EoM}
\end{equation}
which is equivalent to:
\begin{equation}
u_k'' + \l[k^2 - \frac{(a^{-m})''}{a^{-m}} \r] u_k = 0
\end{equation}
We are dealing here with the initial conditions of the perturbations which means we are deep in the radiation dominated era. The equation of state is thus $\omega=\frac{1}{3}$. As a consequence:

\begin{align}
& \varepsilon = \frac{n}{2}-1 = \frac{1}{2}(n-2) \\
& m = \frac{2}{n}-1 \\
& a(\eta) = \eta^\frac{n}{2-n}
\end{align}

Eq.\eqref{EoM} becomes:

\begin{equation}
\boxed{u_k'' + \l[k^2 - 2 \eta^{-2} \r] u_k = 0}
\end{equation}

\end{document}
