# Supplementary material for: CMB Tensor Anisotropies in f(R) Gravity
Source: arXiv:1302.1887 source file (2013-02-07)
Supplement: Supplementary file 2 [file manifolds.tex]

The metric tensor is one very important, if not the most important, structure defined on a manifold:
\begin{equation}
g_{ab} \equiv \vec e_a \cdotp \vec e_b
\label{metric}
\end{equation}
where the vectors $\vec e_a$ are the basis of the manifold.

The covariant derivative on the manifold:
\begin{equation}
T_{abc\cdots;z} = T_{abc\cdots,z} - \Gamma^k_{\phantom kaz} T_{kbc\cdots}  - \Gamma^k_{\phantom kbz} T_{akc\cdots} - \cdots
\end{equation}
obviously requires the \emph{affine connection} \cite{Clifton:2011jh}:
\begin{equation}
\Gamma^a_{\phantom abc} \equiv  \{^a_{bc}\} + K^a_{\phantom abc} + L^a_{\phantom abc}
\label{Gamma} 
\end{equation}
where $\{^a_{bc}\}$ is the Levi-Civita connection defined in terms of the metric tensor:
\begin{equation}
\{^{a}_{bc}\} \equiv \frac{1}{2} g^{ad} (g_{bd,c} + g_{cd,b} - g_{bc,d})
\label{LCC} 
\end{equation}
$K^a_{\phantom a b c}$ is the contorsion tensor defined in terms of the anti-symmetric parts of the connection:
\begin{equation}
K^a_{\phantom a b c} \equiv \Gamma^a_{\phantom a [b c]} - \Gamma^d_{\phantom d [b e]} g^{ae} g_{cd} - \Gamma^d_{\phantom d [c e]} g^{ae} g_{bd}
\label{contorsion} 
\end{equation}
or in terms of the torsion tensor $T_{ab}^{\phantom{ab}c} \equiv 2 \Gamma^c_{\phantom c [ab]}$ \cite{ortin2007}:
\begin{equation}
K_{ab}^{\phantom{ab}c} \equiv \frac{1}{2} g^{cd} \l( T_{adb} + T_{bda} - T_{abd} \r) 
\label{contorsion2} 
\end{equation}
Finally, $L^a_{\phantom a b c}$ is defined in terms of the non-metricity tensor, $Q_{abc} \equiv \nabla_a g_{bc}$, as:
\begin{equation}
L^a_{\phantom a b c} \equiv \frac{1}{2} \l( Q^a_{\phantom a cb} - Q_{bc}^{\phantom{bc}a} - Q_{cb}^{\phantom{cb}a} \r) 
\label{contorsion2} 
\end{equation}

The GR spacetime is a four dimensional torsionless manifold that satisfies the \emph{metric postulate} $Q_{abc} = 0$. That is to say that both $K^a_{\phantom a b c}$ and $L^a_{\phantom a b c}$ vanish and the connection, which is now symmetric on the lower indices, reduces to the Levi-Civita connection which is completely defined by the metric tensor.

The curvature of a region on a manifold is described by the change of the order of the double covariant differentiation of a vector field:
\begin{equation}
v_{a;bc} - v_{a;cb} = R^d_{\phantom dabc} v_d
\label{vector_curv}
\end{equation}
where
\begin{equation}
R^d_{\phantom dabc} \equiv \Gamma^d_{\phantom dac,b} - \Gamma^d_{\phantom dab,c} + \Gamma^e_{\phantom eac} \Gamma^d_{\phantom deb} - \Gamma^e_{\phantom eab} \Gamma^d_{\phantom dec}
\end{equation}
is called the \emph{Riemann tensor} or the \emph{curvature tensor}, which obeys the following symmetries in the metric connection:
\begin{align}
& R_{abcd} = R_{cdab} &&\mathrm{Symmetry\ over\ the\ first\ and\ last\ pair\ of\ indices} \label{Riemann_sym}\\
& R_{abcd} = R_{[ab][cd]} &&\mathrm{Antisymmetry\ in\ the\ first\ and\ last\ pair\ of\ indices} \label{Riemann_anti_sym}\\
& R_{a[bcd]} = 0 &&\mathrm{Cyclic\ identities} \label{cyclic_id} \\
& R_{[ab|cd|;e]} = 0 &&\mathrm{Bianchi\ identities} \label{bianchi_id} 
\end{align}
The Bianchi identities are derived from the cyclic identities. Equation \eqref{vector_curv} is an important geometrical result for 4-vectors that will be used in deriving the Raychaudhuri equation \eqref{raychaudhuri}.

Contraction over the first and third indices of the Riemann tensor yields another curvature tensor dubbed the \emph{Ricci tensor}:
\begin{equation}
R_{ab} \equiv g^{cd} R_{cadb} = R^c_{\phantom cacb}
\end{equation}
Another contraction over the two indices of the Ricci tensor gives the \emph{Ricci scalar}:
\begin{equation}
R \equiv g^{ab} R_{ab} = R^a_a
\end{equation}
defined at every point of the manifold.

It is worth finishing by stating a relation of great importance in relativity. From the Bianchi identities (Eq. \ref{bianchi_id}), and using the symmetry relation (Eq. \ref{Riemann_anti_sym}) it follows that:
\begin{equation}
\l( R_{ab} - \frac{1}{2} g_{ab} R \r)^{;b} = 0
\end{equation}
The Einstein tensor $G_{ab} \equiv R_{ab} - \frac{1}{2} g_{ab} R$ is divergence free \cite{Hobson}.
