# Supplementary material for: CMB Tensor Anisotropies in f(R) Gravity
Source: arXiv:1302.1887 source file (2013-02-07)
Supplement: Supplementary file 6 [file custom_commands.tex]

%%%%%%%%%%%%%%%%%%%% % Bourhrous % %%%%%%%%%%%%%%%%%%%%%%
\def \vec #1{\textbf{\em  #1}}
\newcommand{\Cl}{C_\ell}
\newcommand{\Pl}{P_\ell}
\newcommand{\cn}{/**citation needed**/}
%\newcommand{\l}{\ell}
%%%%%%%%%%%%%%%% % Leong % %%%%%%%%%%%%%%%%

\newcommand{\p}{\partial}
%\newcommand{\g}{\gamma}
\newcommand{\D}{\Delta}
\newcommand{\n}{\nabla}
\def\l{\left}
\def\r{\right}
\def\D{\Delta}
\def\dt{\cdot}
\def\w{\wedge}
\def\n{\nabla}
\newcommand{\hs}{\,-\,}
\newcommand \dd[2] {\frac{d {#1}}{d {#2}}}
\newcommand \pp[2] {\frac{\p {#1}}{\p {#2}}}
\newcommand \ppd[2] {\frac{\p^2 {#1}}{\p {#2}^2}}
\newcommand \ddp[2] {\frac{ d^2 {#1}}{d {#2}^2}}
\newcommand \bra[1] {\big< {#1}|}
\newcommand \ket[1] {| {#1} \big>}
\newcommand \ps {\mathcal{I}}
\newcommand{\nab}{\tilde{\nabla}}
\renewcommand{\theequation}{\arabic{equation}}
\def\mat#1  { \begin{matrix}#1\end{matrix} }
\def\pmat#1 { \begin{pmatrix}#1\end{pmatrix} }
\def\cas#1  { \begin{cases}#1\end{cases} }

%%%%%%%%%%%%%%%%% Commands from Ananda et. al %%%%%%%%%%%%
% 

\def \D {\tilde{\nabla}}
\def \ni {\noindent}
% \def\l{\label}
% \def\ct{\cite}
% \def\r{\ref}
% \def\lgth{[\,\mbox{length}\,]}
% \def\gam{\gamma}
% \def\del{\delta}
% \def\eps{\Epsilon}
% \def\Th{\Theta}
% \def\dd{\mathcal D}
% \def\zz{\mathcal Z}
% \def\sig{\sigma}
% \def\om{\omega}
% \def\udot{\dot{u}}
% \def\nab{\nabla}
\def\3nab{\tilde{\nabla}}
% \def\fd{{\bf e}}
% \def\p{\partial}
\def\lgl{\langle}
\def\rgl{\rangle}
% \def\la {\langle}
% \def\ra {\rangle}
\def\nn{\nonumber}
\def\c{\mbox{curl}}
% \def\div{\mbox{div}}
% \def\tl{\tilde}
% \def\hsp5{\hspace{5mm}}
% \newcommand{\sfrac}[2]{{\textstyle{#1\over#2}}}
% \def\case#1/#2{\textstyle\frac{#1}{#2}}
% \def\rd {\displaystyle{\cdot}}
% \def\ts {\textstyle}
% \def\be {\begin{equation}}
% \def\ee {\end{equation}}
% \def\ber {\begin{eqnarray}}
% \def\eer {\end{eqnarray}}
% \def\bea {\begin{eqnarray}}
% \def\eea {\end{eqnarray}}
% \def\cs{c_{s}^{2}}
% \def\ub {u_{\!_B}}
% \def\vb {v_{\!_B}}
% \def\eb {e_{\!_B}}
% \def\st {\sigma_{\!_T}}
% \def\ne {n_{\!_E}}
% \def\ts {\textstyle}
% \def\bc {\begin{center}}
% \def\ec {\end{center}}
% \newcommand{\hs}{\,-\,}
% \def\bi {\bibitem}
% %\def\case#1/#2{\textstyle\frac{#1}{#2} }
% \def\t {\textstyle}
% \def\jmp{{\it J. Math. Phys.}\ }
% \def\pr{{\it Phys. Rev.}\ }
% \def\jmp{{\it J. Math. Phys.}\ }
% \def\pr{{\it Phys. Rev.}\ }
% \def\prl{{\it Phys. Rev. Lett.}\ }
% \def\pl{{\it Phys. Lett.}\ }
% \def\np{{\it Nucl. Phys.}\ }
% \def\modpl{{\it Mod. Phys. Lett.}\ }
% \def\ijmp{{\it Int. Journ. Mod. Phys.}\ }
% \def\ijtp{{\it Int. Journ. Theor. Phys.}\ }
% \def\cmp{{\it Commun. Math. Phys.}\ }
% \def\cqg{{\it Class. Quantum Grav.}\ }
% \def\ap{{\it Ann. Phys. (N.Y.)}\ }
% \def\spj{{\it Sov. Phys. JETP}\ }
% \def\spjl{{\it Sov. Phys. JETP Lett.}\ }
% \def\prs{{\it Proc. R. Soc.}\ }
% \def\grg{{\it Gen. Relativ. Grav.}\ }
% \def\nat{{\it Nature}\ }
% \def\apj{{\it Ap. J.}\ }
% \def\aa{{\it Astron. Astrophys.}\ }
% \def\ncim{{\it Il Nuovo Cim.}\ }
% \def\ptp{{\it Prog. Theor. Phys.}\ }
% \def\aip{{\it Adv. Phys.}\ }
% \def\jpamg{{\it J. Phys. A: Math. Gen.}\ }
% \def\mnras{{\it Mon. Not. R. Ast. Soc.}\ }
% \def\prep{{\it Phys. Rep.}\ }
% \def\ncb{{\it Il Nuovo Cimento ``B''}}
% \def\ssr{{\it Space Sci. Rev.}\ }
% \def\pasp{{\it Pub. A. S. P.}\ }
% \def\araa{{\it Ann. Rev. Astr. Ap.}\ }
% \def\asr{{\it Adv. Space Res.}\ }
% \def\rmp{{\it Rev. Mod. Phys.}\ }
% \def\etal\;{{\it et al.}}
% \def\ie{{\it i.e. }}
% \def\eg{{\it e.g. }}
% \def\jmp{{\it J. Math. Phys.}\ }
% \def\lrr{{\it Liv. Rev. Rel.}\ }
% \def\nat{{\it Nature}\ }
% \def\apj{{\it Ap. J.}\ }
% \def\mnras{{\it Mon. Not. R. Ast. Soc.}\ }
% \def\araa{{\it Ann. Rev. Astr. Ap.}\ }
% \def\rmp{{\it Rev. Mod. Phys.}\ }
% \def\arns{{\it Ann. Rev. Nucl. Part. Sci.}\ }
% \newcommand{\n}{{}^{(3)}\nabla} \newcommand{\na}{\nabla}
% \newcommand{\hl}{\vspace{0.2cm}\hrule width\hsize height 0.45pt\vspace{0.2cm}}
% \newcommand{\da}{{\cal D}_a}
% \newcommand{\ft}{\left(\frac{t}{t_i}\right)}
% \newcommand{\0}{^{(0)}}
% \newcommand{\1}{^{(1)}}
% \newcommand{\2}{^{(2)}}
% \newcommand{\ab}{_{\alpha\beta}}
% \newcommand{\h}{\case{a'}/{a}}
% \newcommand{\inps}{\psi^{-1}}
% \newcommand{\ua}{\left(\frac{\nabla_a\phi}{\psi}\right)}
% \newcommand{\as}{{\cal A}}
% \newcommand{\bb}{{\cal B}}
% \newcommand{\cc}{{\cal C}}
% \newcommand{\es}{{\cal E}}
% \newcommand{\kk}{{\cal K}}
% \newcommand{\ls}{{\cal L}}
% \newcommand{\so}{{\cal O}}
% \newcommand{\sr}{{\cal R}}
% \newcommand{\ti}{\tilde}
% \newcommand{\wt}{\widetilde}
% \newcommand{\ii}{{(i)}}
% \newcommand{\jn}{{(j)}}
% \newcommand{\wcn}{\wt{C}_{(\nu)}}
% \newcommand{\dn}{\Delta_{(\nu)}}
% \newcommand{\pn}{\Phi_{(n)}}

% Challinor
\newcommand{\curl}{\,\mbox{curl}\,}
% \newcommand{\ord}{\mbox{O}}
% \newcommand{\sigt}{\sigma_{\mathrm{T}}}
% \newcommand{\nelec}{n_{\mathrm{e}}}
% \newcommand{\ud}{{\mathrm{d}}}
\newcommand{\Drm}{{\mathrm{D}}}
% \newcommand{\tc}{t_{\mathrm{c}}}
% \newcommand{\clq}{{\mathcal{Q}}}
% \newcommand{\TT}{{\mathrm{TT}}}
% \newcommand{\clh}{{\mathcal{H}}}
% \newcommand{\clp}{{\mathcal{P}}}
